# Supplementary material for: TinyChirp: Bird Song Recognition Using TinyML Models on Low-power Wireless Acoustic Sensors
Source: arXiv:2407.21453 source file (2024-09-11)
Supplement: Supplementary file 1 [file 99-appendix.tex]

\section*{Appendix}

\todo[inline]{model training details, hyperparameters etc.}

\begin{table}[]
    \centering
    \caption{Hyperparameters for training \ac{TinyML} models.}
    \begin{tabular}{ll}
    \toprule
     Parameter  & Value \\
     \midrule
     Random Seed    &  \\
     Epoch & \\
     Optimizer & \\
     Learning Rate & \\
     Batch Size & \\
     Loss & \\
     Penalty & \\

    \bottomrule
    \end{tabular}
    
    \label{tab:hyper_param_training}
\end{table}
